# Supplementary material for: Exotic Gapless Mott Insulators of Bosons on Multi-Leg Ladders
Source: arXiv:1008.4105 ancillary file (2011-01-28)
Supplement: Supplementary file 1 [file GapsSupplement.pdf]

# Supplementary Material to
# Exotic Gapless Mott Insulators of Bosons on Multi-Leg Ladders


Matthew S. Block,[1] Ryan V. Mishmash,[1] Ribhu K. Kaul,[2,3] D. N. Sheng,[4]
Olexei I. Motrunich,[5] and Matthew P. A. Fisher[1,5]

[1]*Department of Physics, University of California, Santa Barbara, CA 93106, USA*
[2]*Microsoft Station Q, University of California, Santa Barbara, CA 93106, USA*
[3]*Department of Physics and Astronomy, University of Kentucky, Lexington, KY 40506, USA*
[4]*Department of Physics and Astronomy, California State University, Northridge, CA 91330, USA*
[5]*Department of Physics, California Institute of Technology, Pasadena, CA 91125, USA*


(Dated: November 28, 2010)


In this document, we focus on the system size dependence of the one-boson gap, two-boson gap, and spectral gap (at fixed number of bosons $M$) in the gapless Mott insulator (GMI) and superfluid (SF) phases as determined by DMRG. We define the $p$-boson gap as

$$\Delta_b^{(p)} = \frac{1}{p}[E_0(M+p) + E_0(M-p) - 2E_0(M)] \tag{1}$$

and the spectral gap as

$$\Delta_{\text{spec}} = E_1(M) - E_0(M), \tag{2}$$

where $E_0(M)$ and $E_1(M)$ are the ground and first excited state energies, respectively, of a system with $M$ bosons. In all cases considered here where the filling factor $\nu = 1/3$, we take $M = L_x$. We consider 3-leg systems of length $L_x = 24, 18, 12, 8$ with fully periodic boundary conditions at the points $K/J = 6.0, 2.7, 1.0$ with $J_\perp/J = 1.0$. The points $K/J = 6.0, 2.7$ are in the GMI phase, while $K/J = 1.0$ is in the superfluid phase; note that $K/J = 2.7$ is the point considered in detail in Fig. 3 of our manuscript.

In Figs. 1 and 2, we see that in the GMI phase $\Delta_b^{(1)}$ and $\Delta_b^{(2)}$ will likely obtain rather large values in the thermodynamic limit, although at these system sizes it is not possible to predict accurately the values of the $L_x \to \infty$ gaps. On the other hand, these gaps clearly scale to zero in the thermodynamic limit in the superfluid phase. These calculations are consistent with the GMI being an incompressible insulator and the superfluid being a compressible fluid.

In Fig. 3, we now plot the spectral gap at fixed boson number for the same points and system sizes. In the superfluid, $\Delta_{\text{spec}}$ again scales linearly to zero with $1/L_x$ in the thermodynamic limit as expected. However, the points in the GMI phase generally have spectral gaps smaller than in the superfluid (even without correcting for the fact that with larger $K$ the natural energy scale of the system is larger for the GMI points; the spectral gap in Fig. 3 is plotted in units of $J$ only), while their scaling with $1/L_x$ is not clear. We expect $\Delta_{\text{spec}}$ to vanish as $L_x \to \infty$ but we generally find it difficult to perform a rigorous finite-size study of these gaps, which we believe is due to the generally incommensurate nature of the projected Fermi sea wave functions when placed on a finite-size system.

Finally, in Fig. 4 we show for completeness how the fixed boson number spectral gap depends on $J_\perp/J$ at fixed $K/J = 6.0$ for various system sizes. This plot elucidates the gapped nature of the rung Mott phase for $J_\perp/J \gtrsim 6.0$, while the points for which $2.0 \lesssim J_\perp/J \lesssim 6.0$ lie within the unidentified phase mentioned in the manuscript (see large white region in our phase diagram, Fig. 2). Even though the properties of physical quantities in this phase are not fully consistent with a GMI state, e.g., lack of power law singularities in the density-density structure factor and scaling of the entanglement entropy inconsistent with $c \simeq 2$, this calculation of the spectral gap indicates that the system is either gapless or has a very small gap in this region.

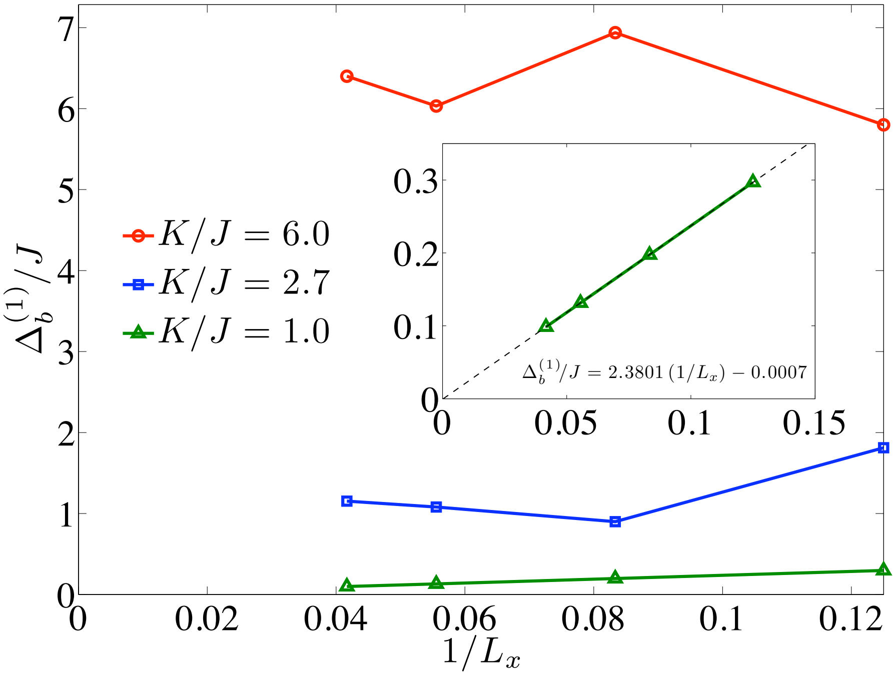


FIG. 1: Finite-size scaling of the one-boson gap $\Delta_b^{(1)}$ at characteristic points in the GMI ($K = 6.0$, $K = 2.7$) and superfluid ($K/J = 1.0$) phases; $J_\perp/J = 1.0$ in all cases. In the inset, we display a linear fit of the superfluid ($K = 1.0$) data.

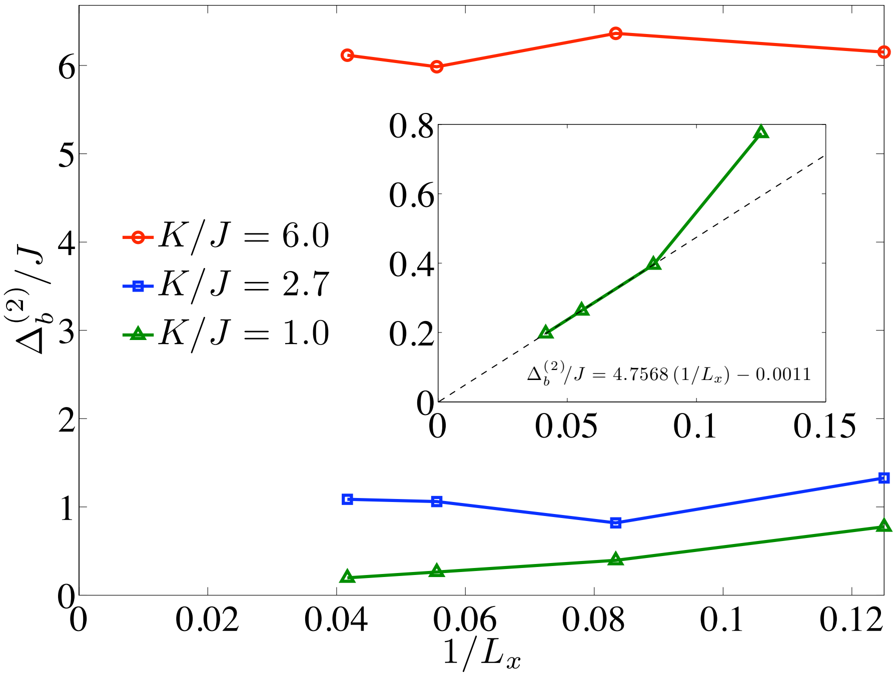


FIG. 2: Finite-size scaling of the two-boson gap $\Delta_b^{(2)}$ at characteristic points in the GMI ($K = 6.0$, $K = 2.7$) and superfluid ($K/J = 1.0$) phases; $J_\perp/J = 1.0$ in all cases. In the inset, we display a linear fit of the superfluid ($K = 1.0$) data, excluding the $L_x = 8$ point.

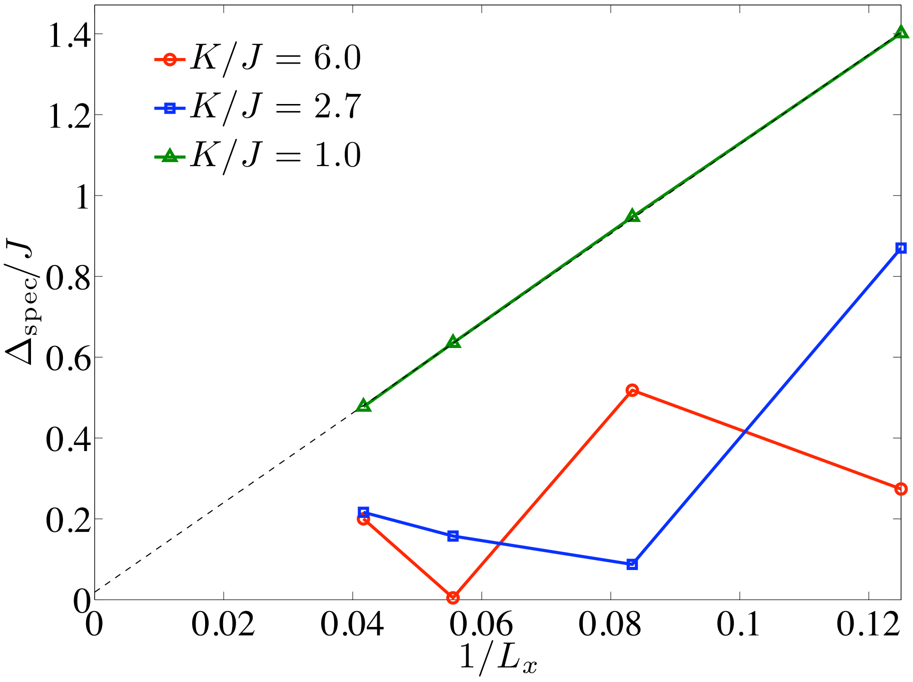


FIG. 3: Finite-size scaling of the spectral gap $\Delta_{\mathrm{spec}}$ at fixed boson number at characteristic points in the GMI ($K = 6.0$, $K = 2.7$) and superfluid ($K/J = 1.0$) phases; $J_\perp/J = 1.0$ in all cases. The dashed black line is a linear fit of the superfluid ($K = 1.0$) data, which is given by $\Delta_{\mathrm{spec}}/J = 11.0815\,(1/L_x) + 0.0187$.

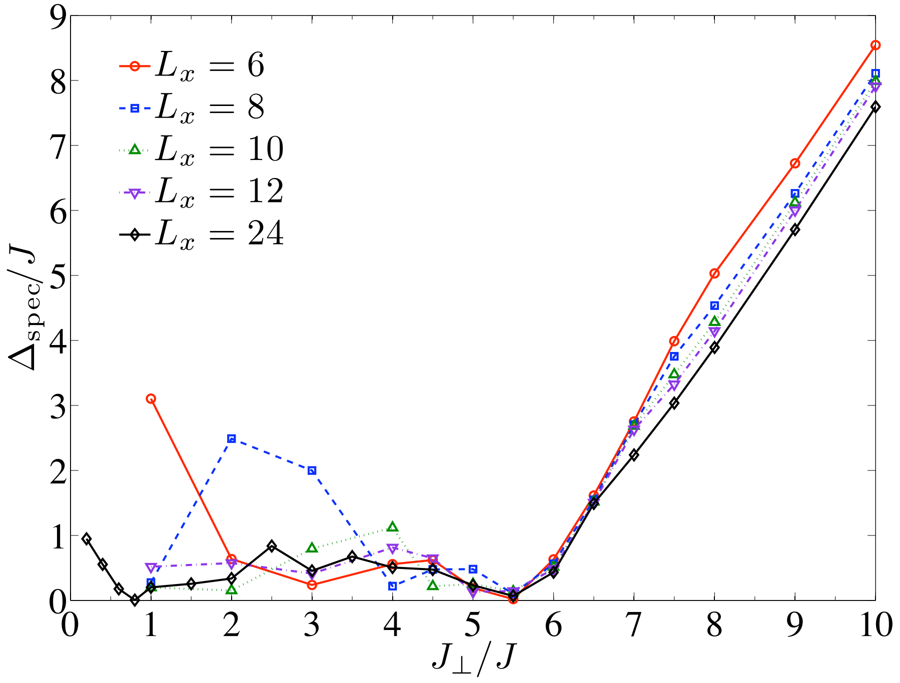


FIG. 4: Dependence of the spectral gap on $J_\perp/J$ at fixed $K/J = 6.0$ at various system sizes $L_x$. For $J_\perp/J \lesssim 2$, we believe the system is in the GMI phase, while for $J_\perp/J \gtrsim 6.0$, the system is in the rung Mott phase. The intermediate region is the unidentified phase as shown in our phase diagram, i.e., Fig. 2 of the manuscript.
